# Supplementary material for: KRONC: Keypoint-based Robust Camera Optimization for 3D Car Reconstruction
Source: arXiv:2409.05407 source file (2024-09-09)

Env1-Fiat

GT

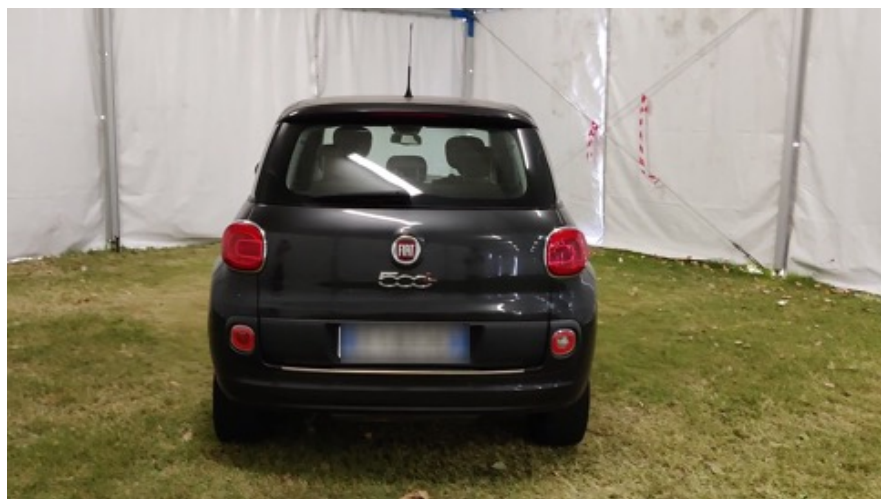

Trajectory

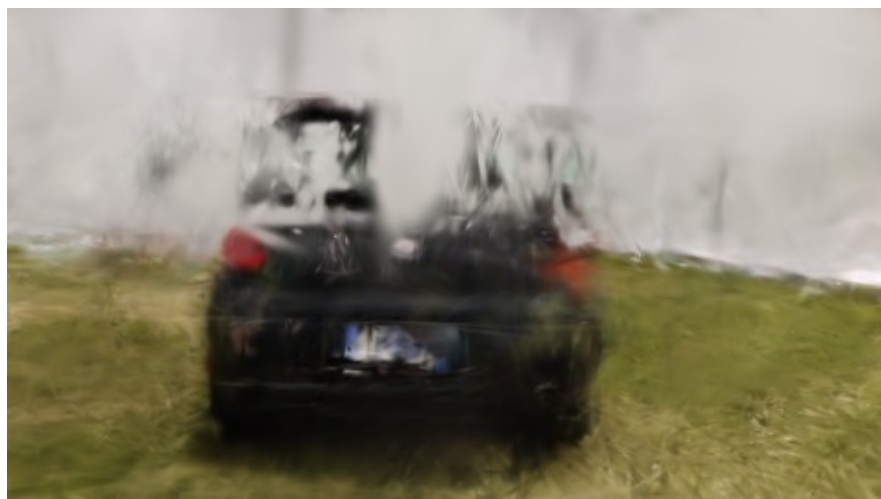

KRONC + GS

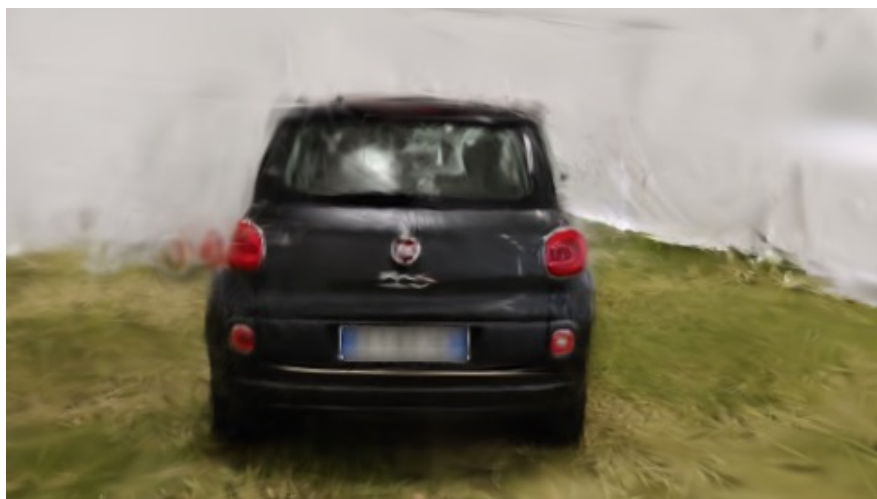

Trajectory

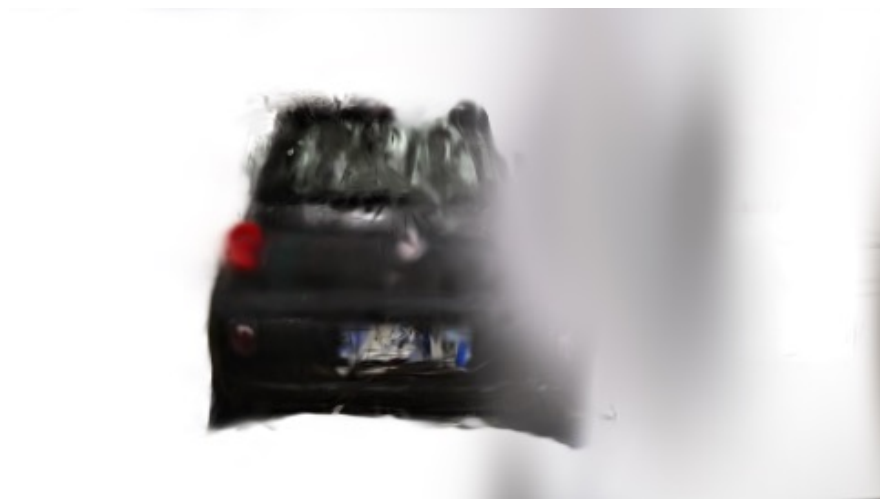

KRONC + GS

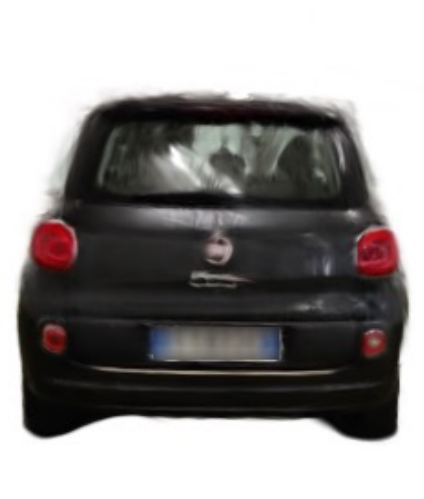

Env1-Ford

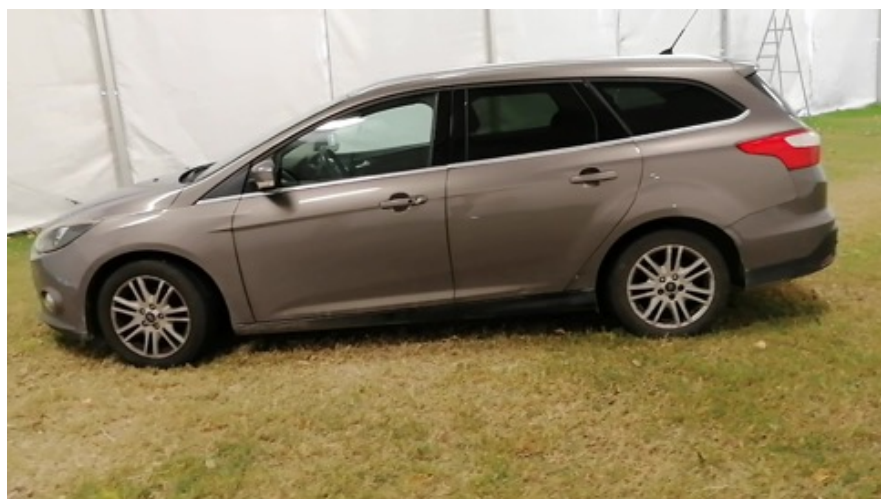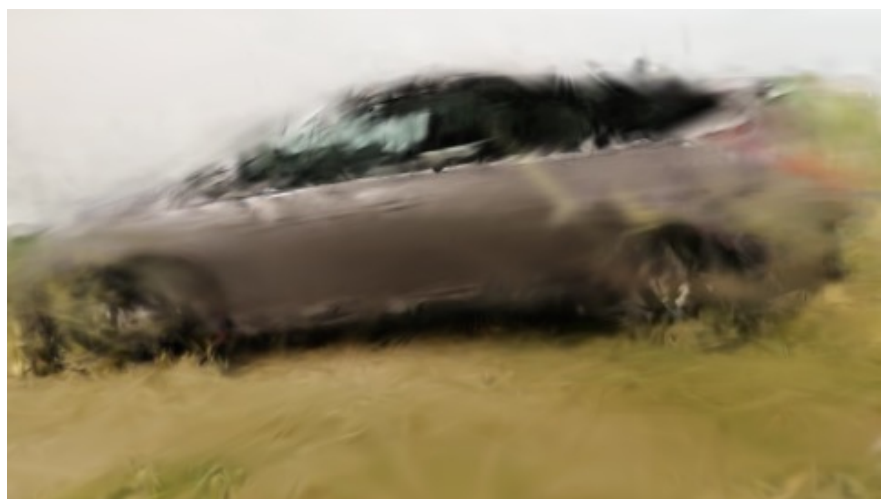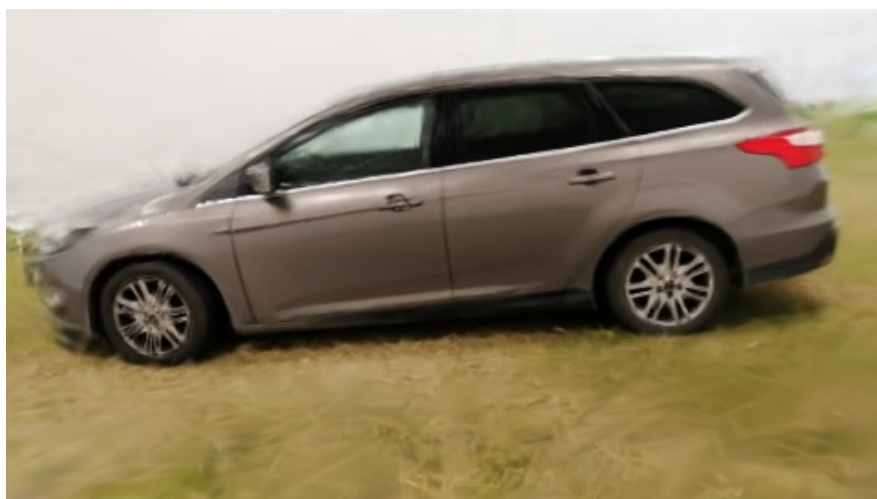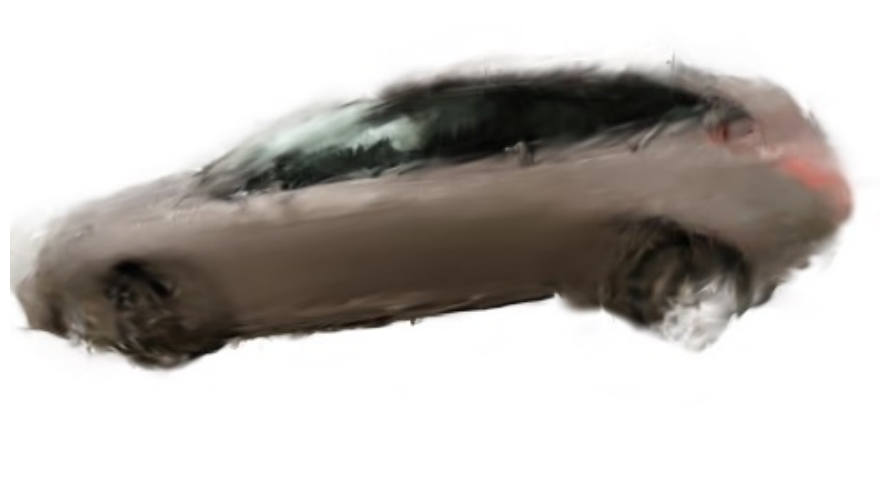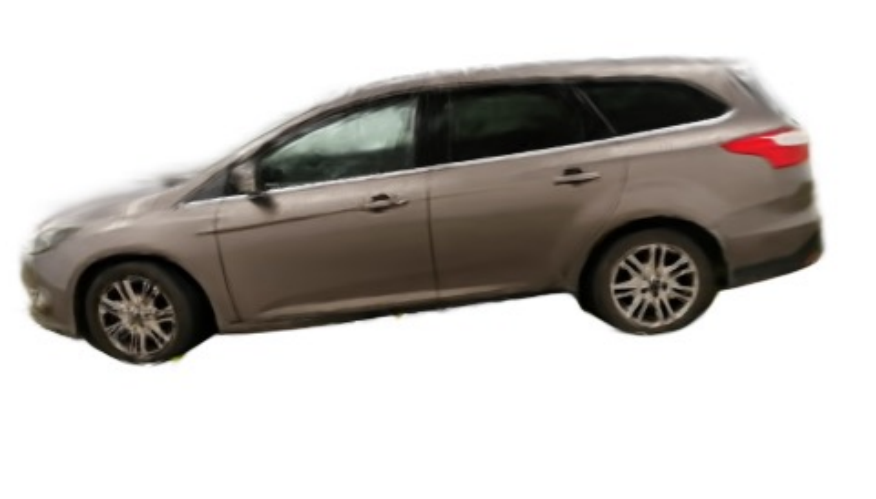

Env1-Hyundai

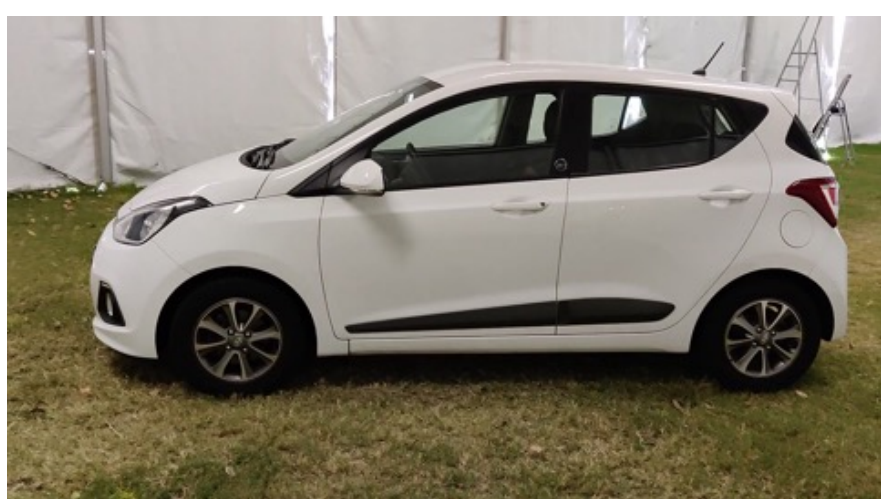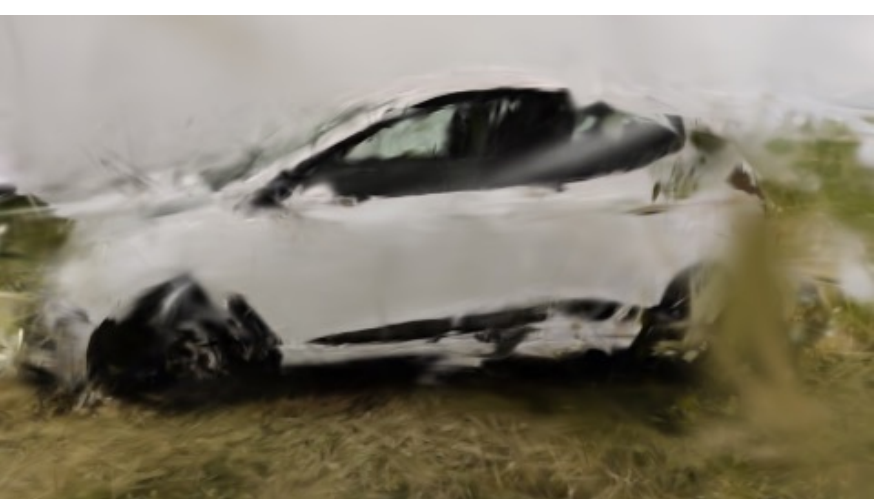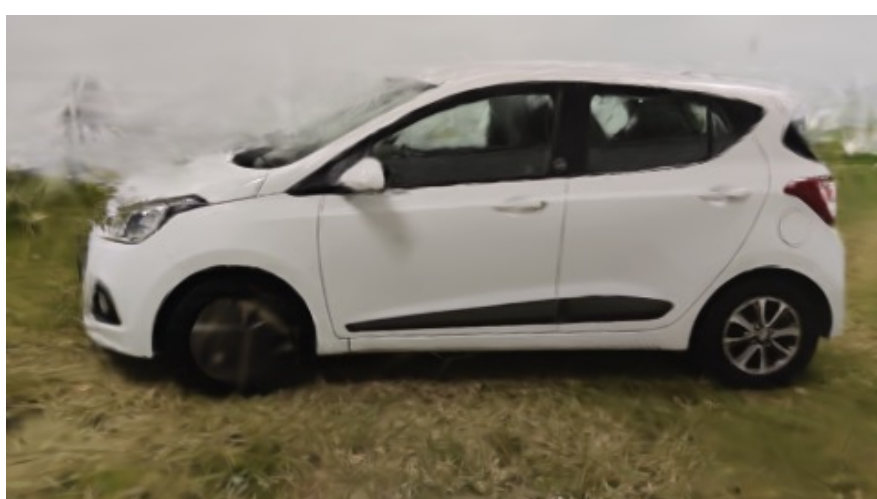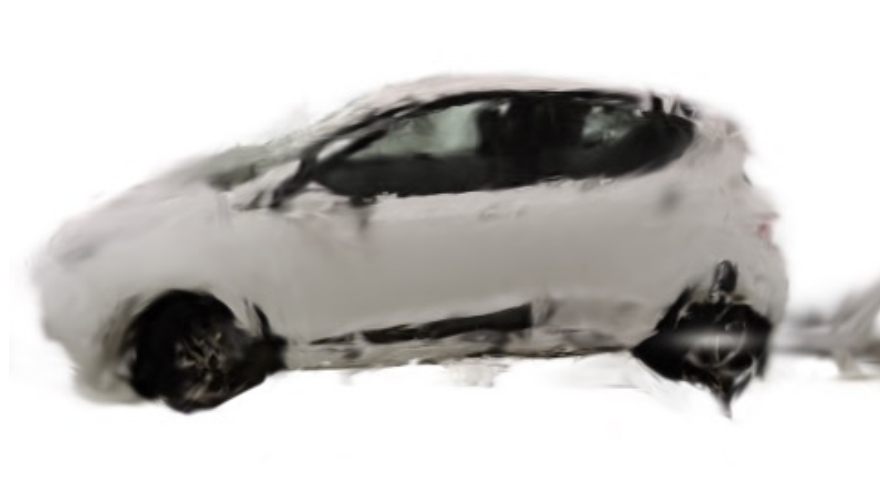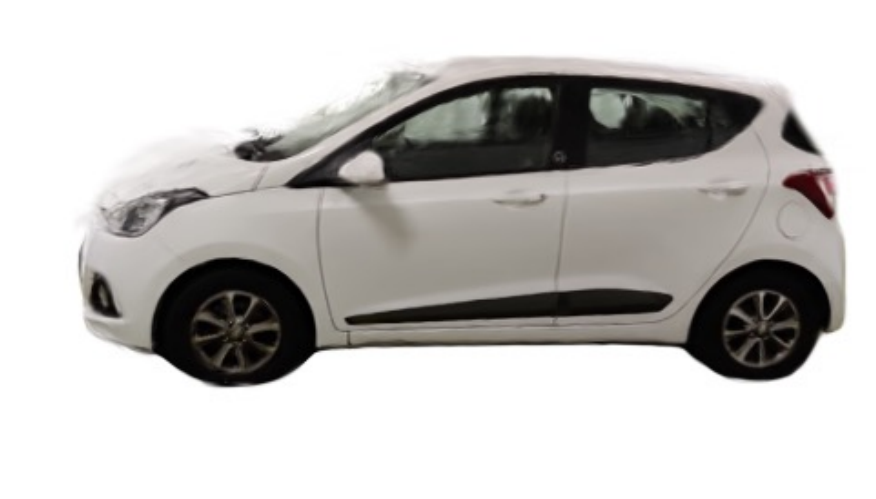

Env2-Yaris

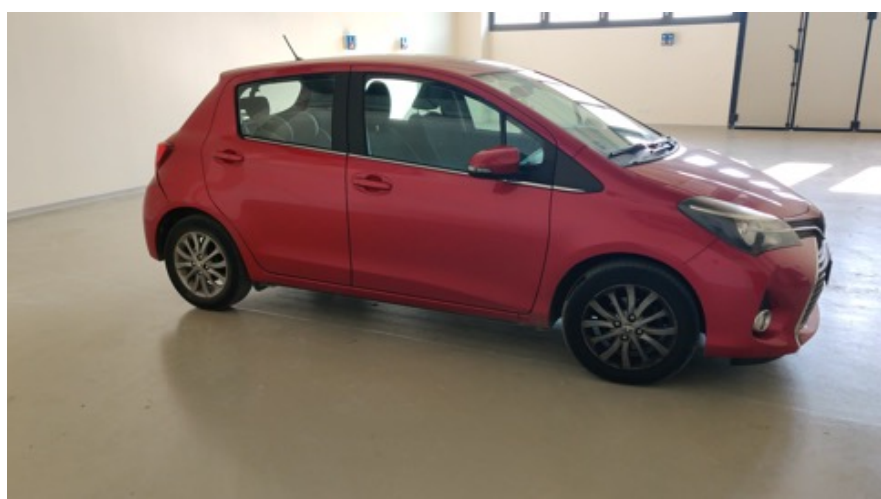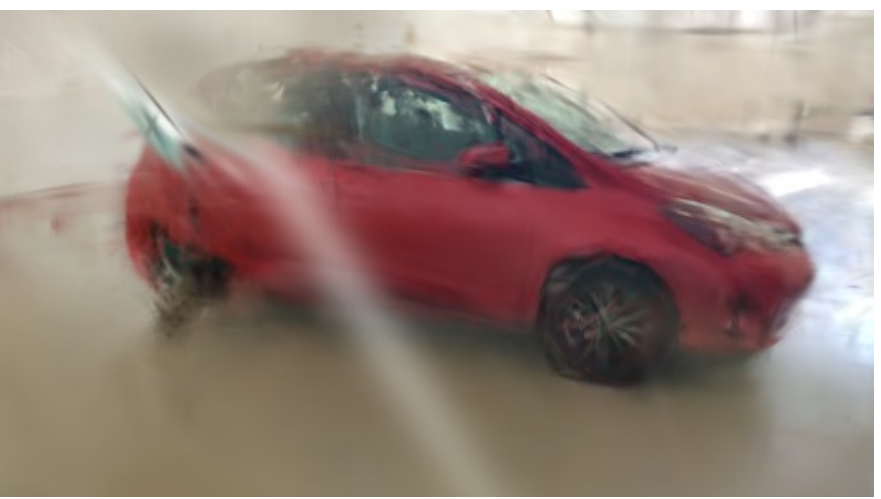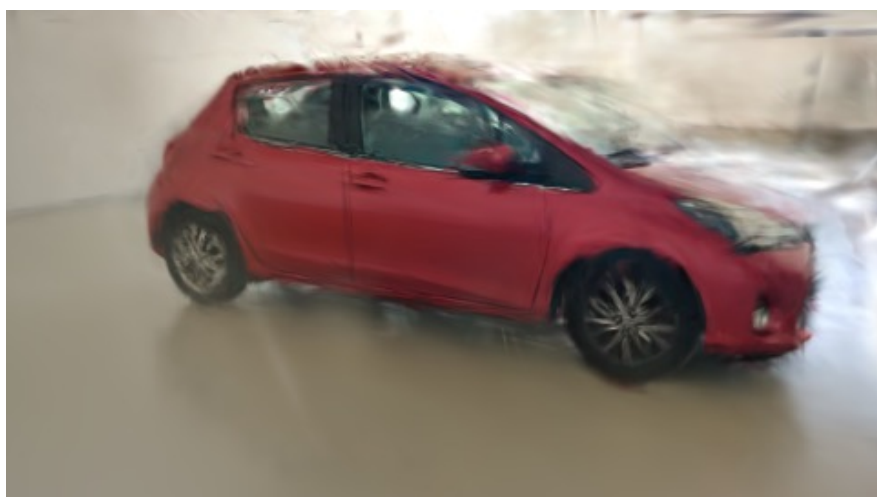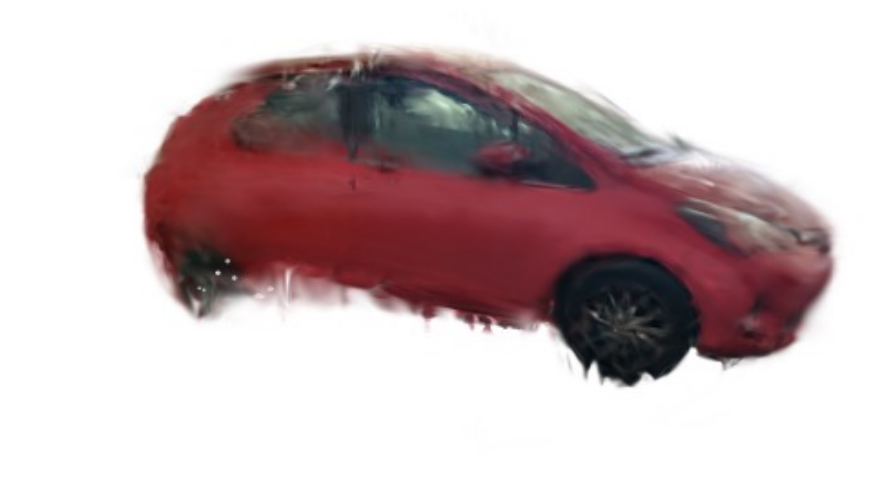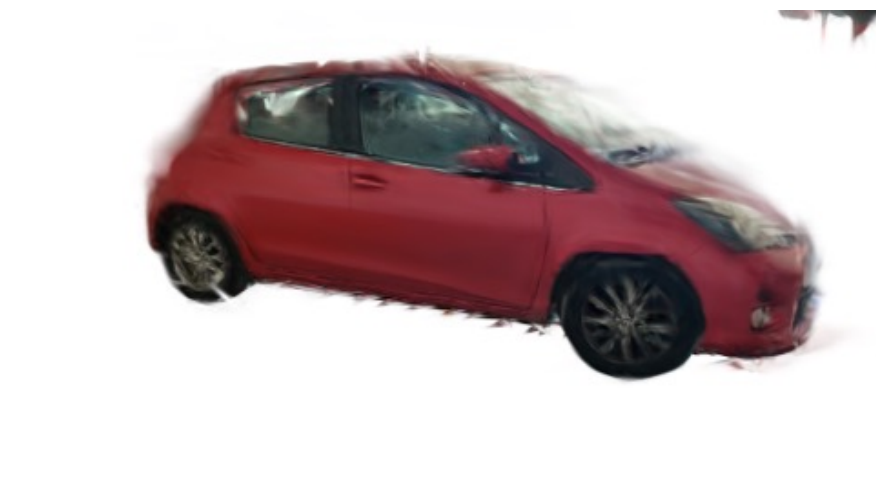



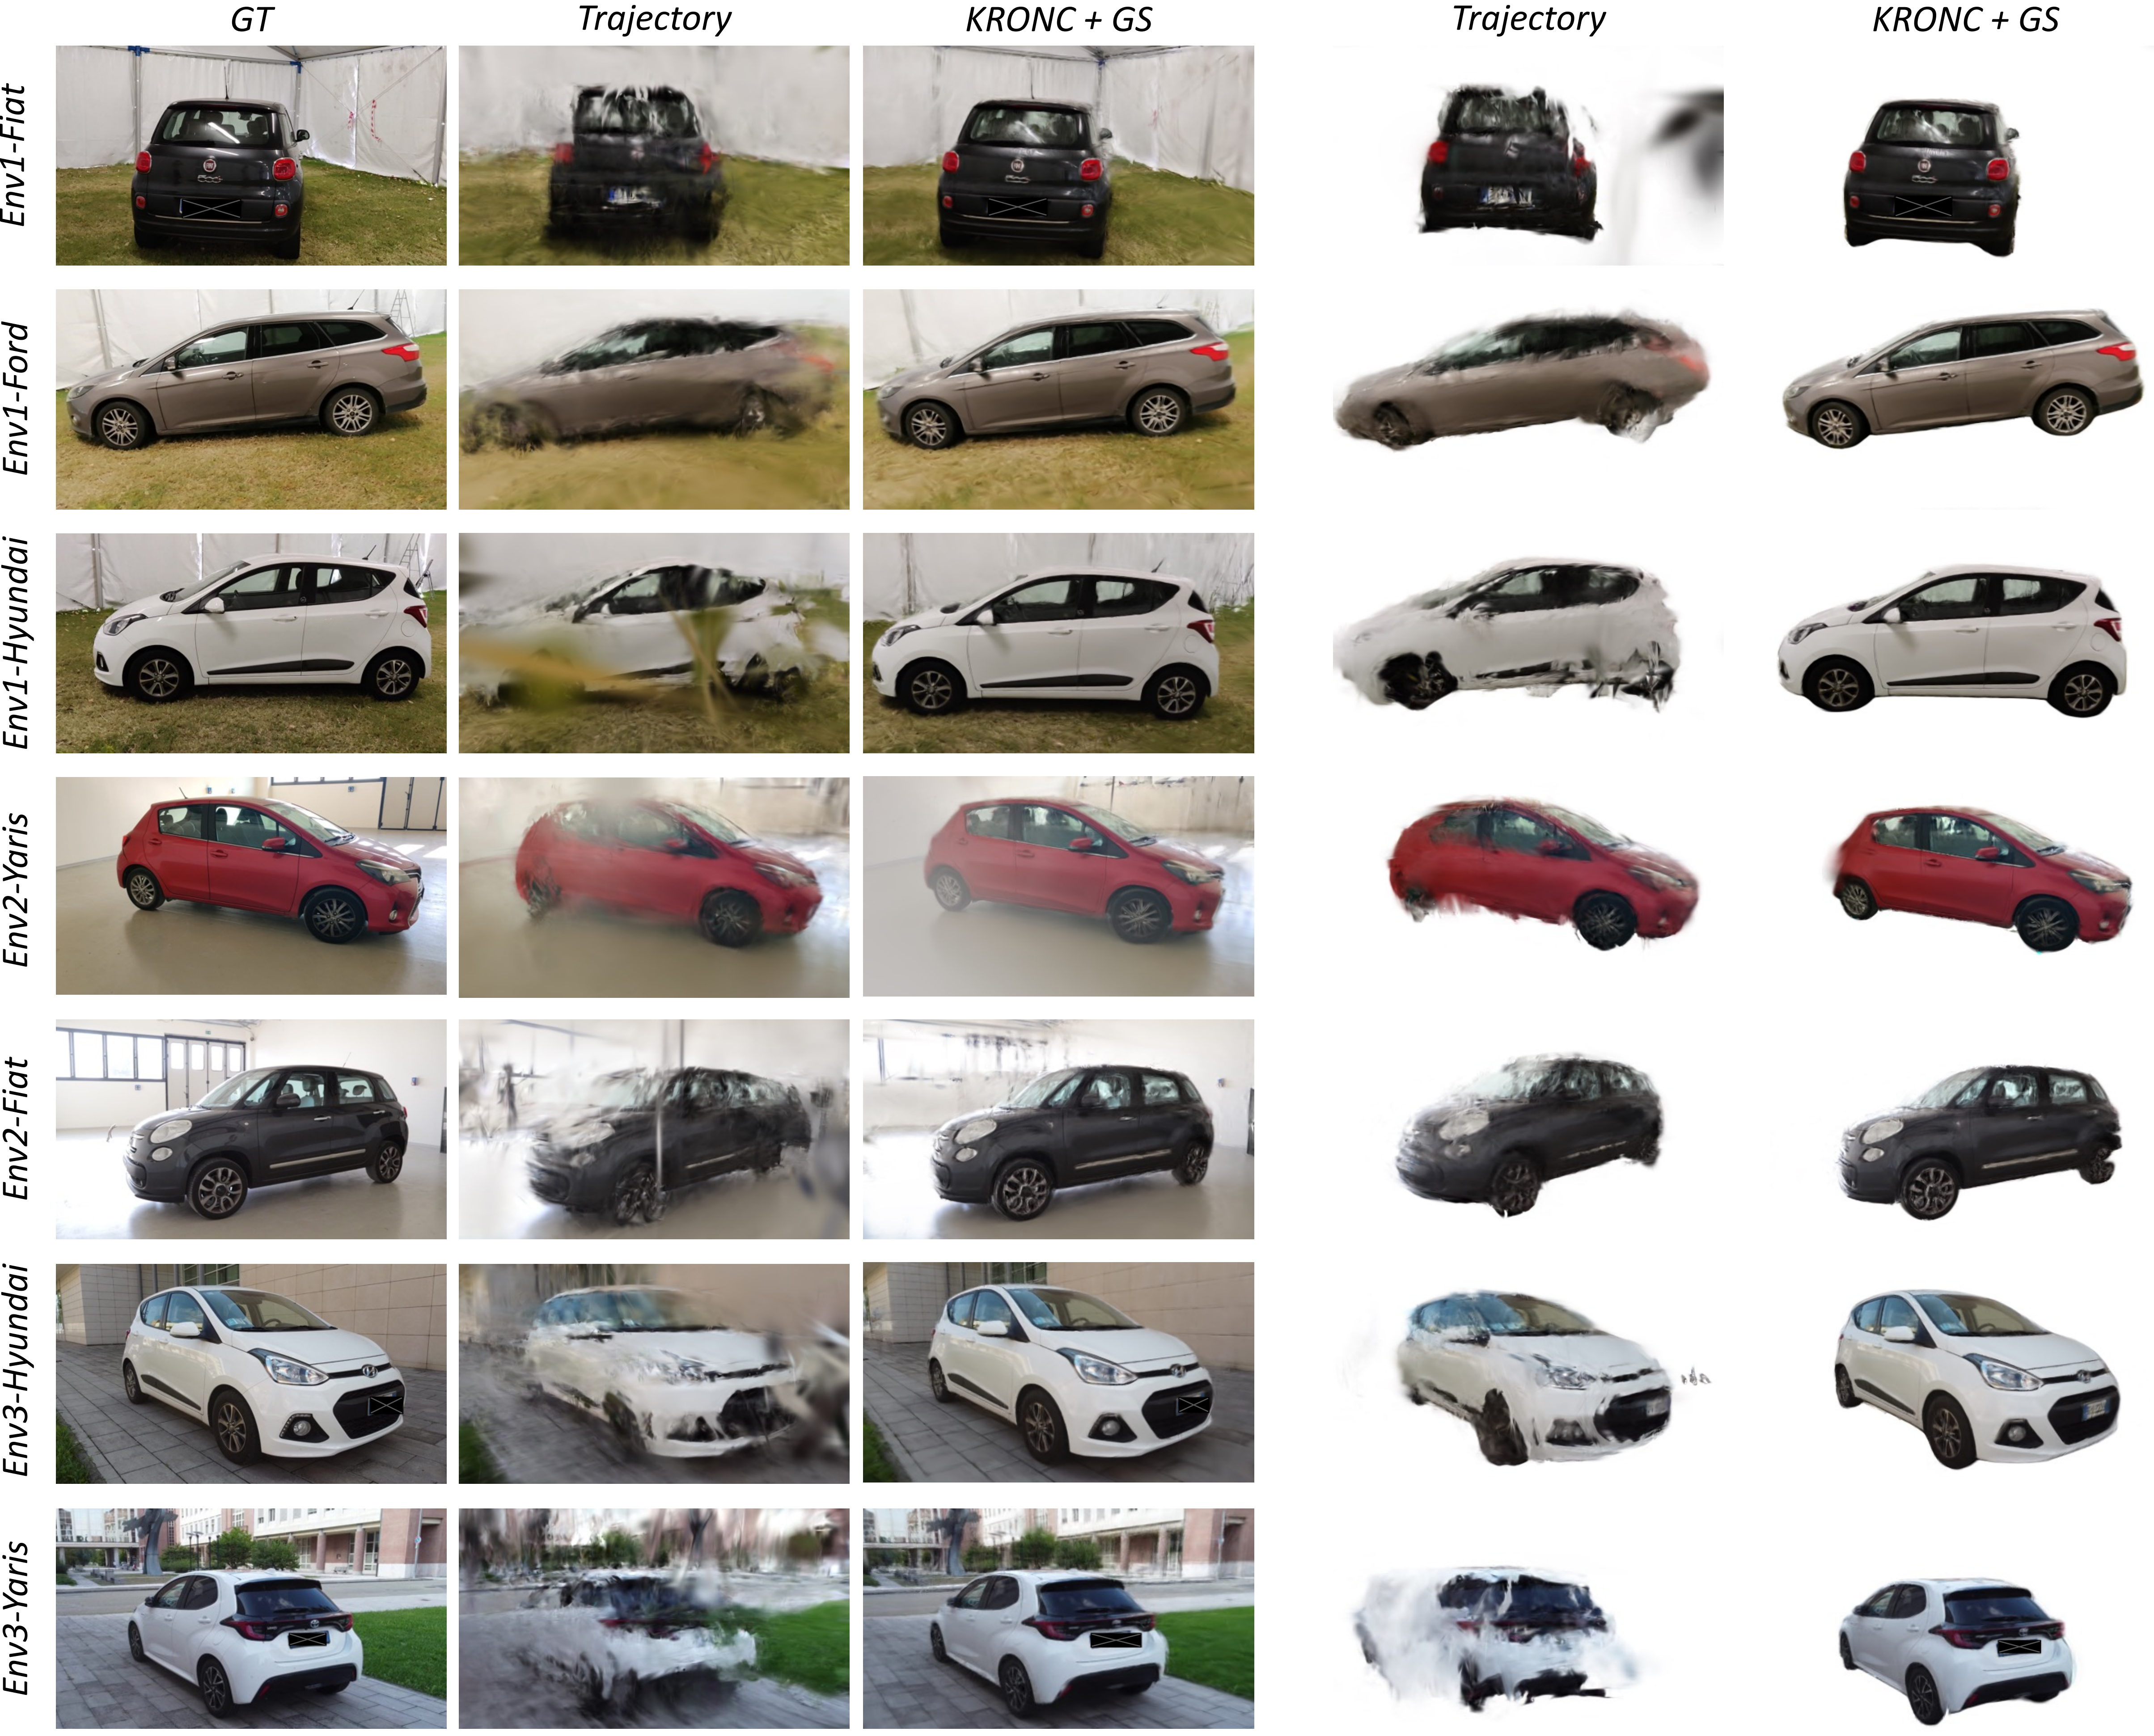

Supplement: Supplementary file 1 [file qualitativi_reale_supp.pdf]
