# Supplementary material for: KRONC: Keypoint-based Robust Camera Optimization for 3D Car Reconstruction
Source: arXiv:2409.05407 source file (2024-09-09)

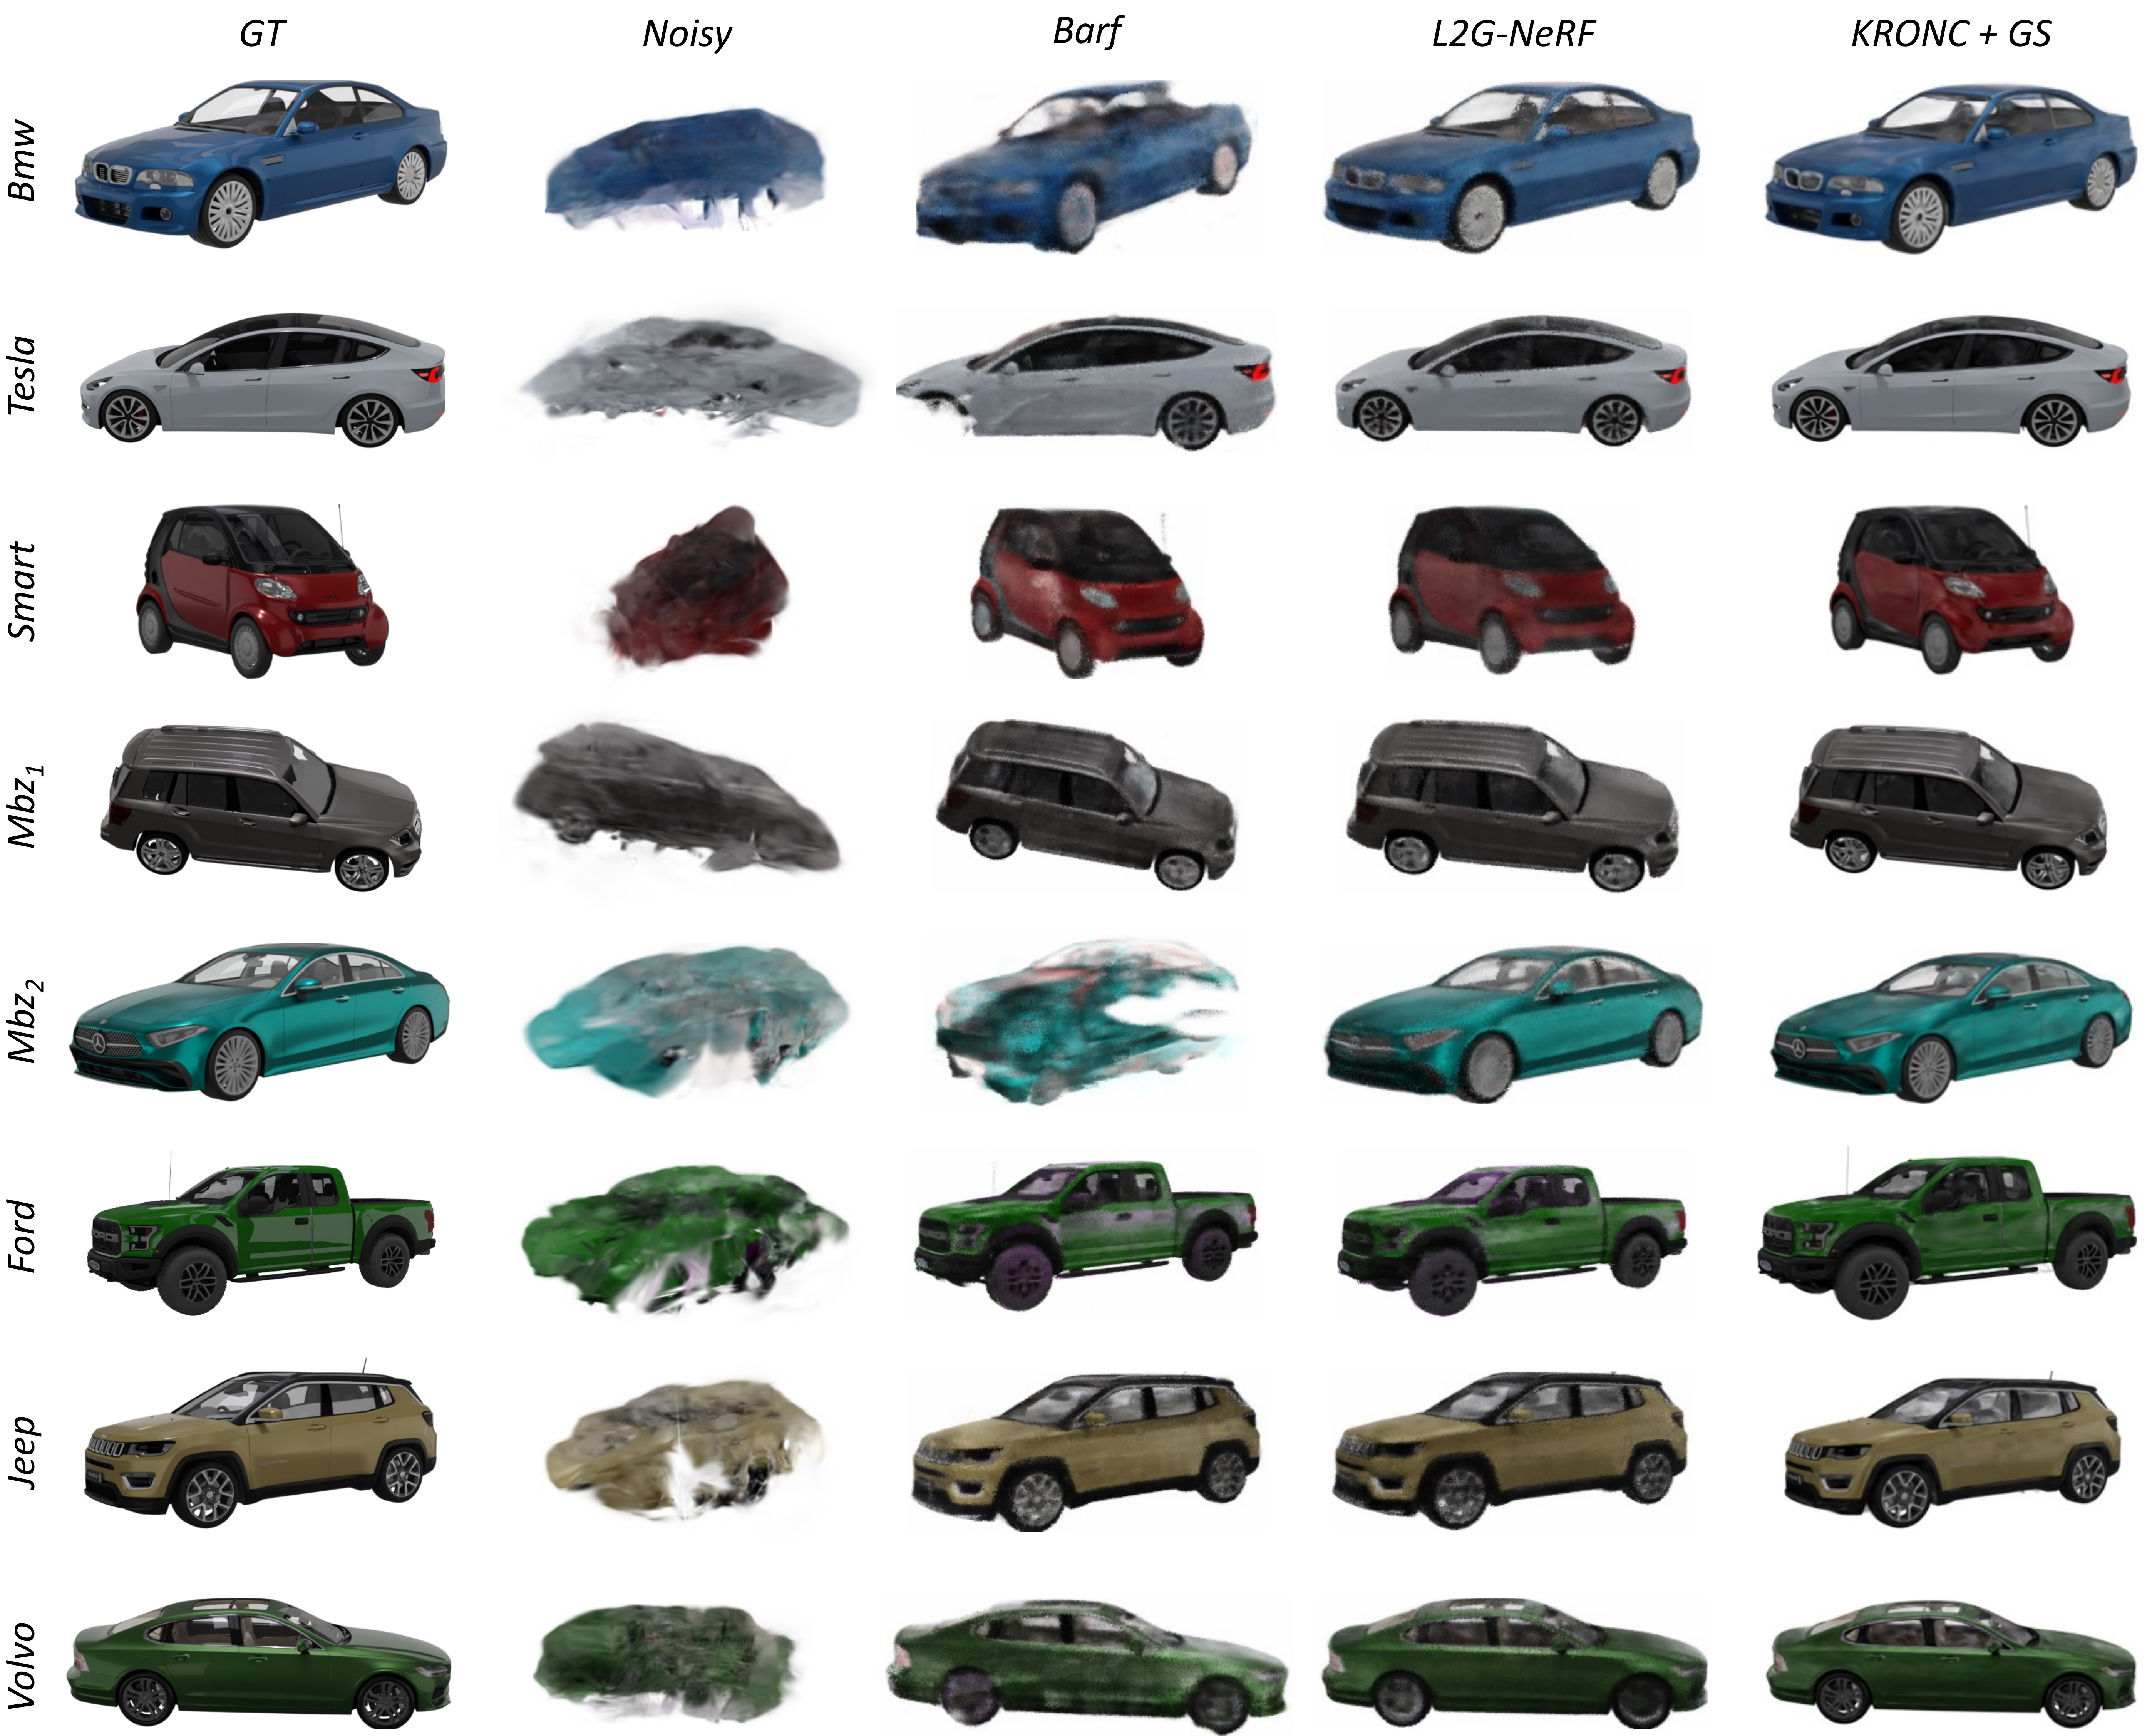

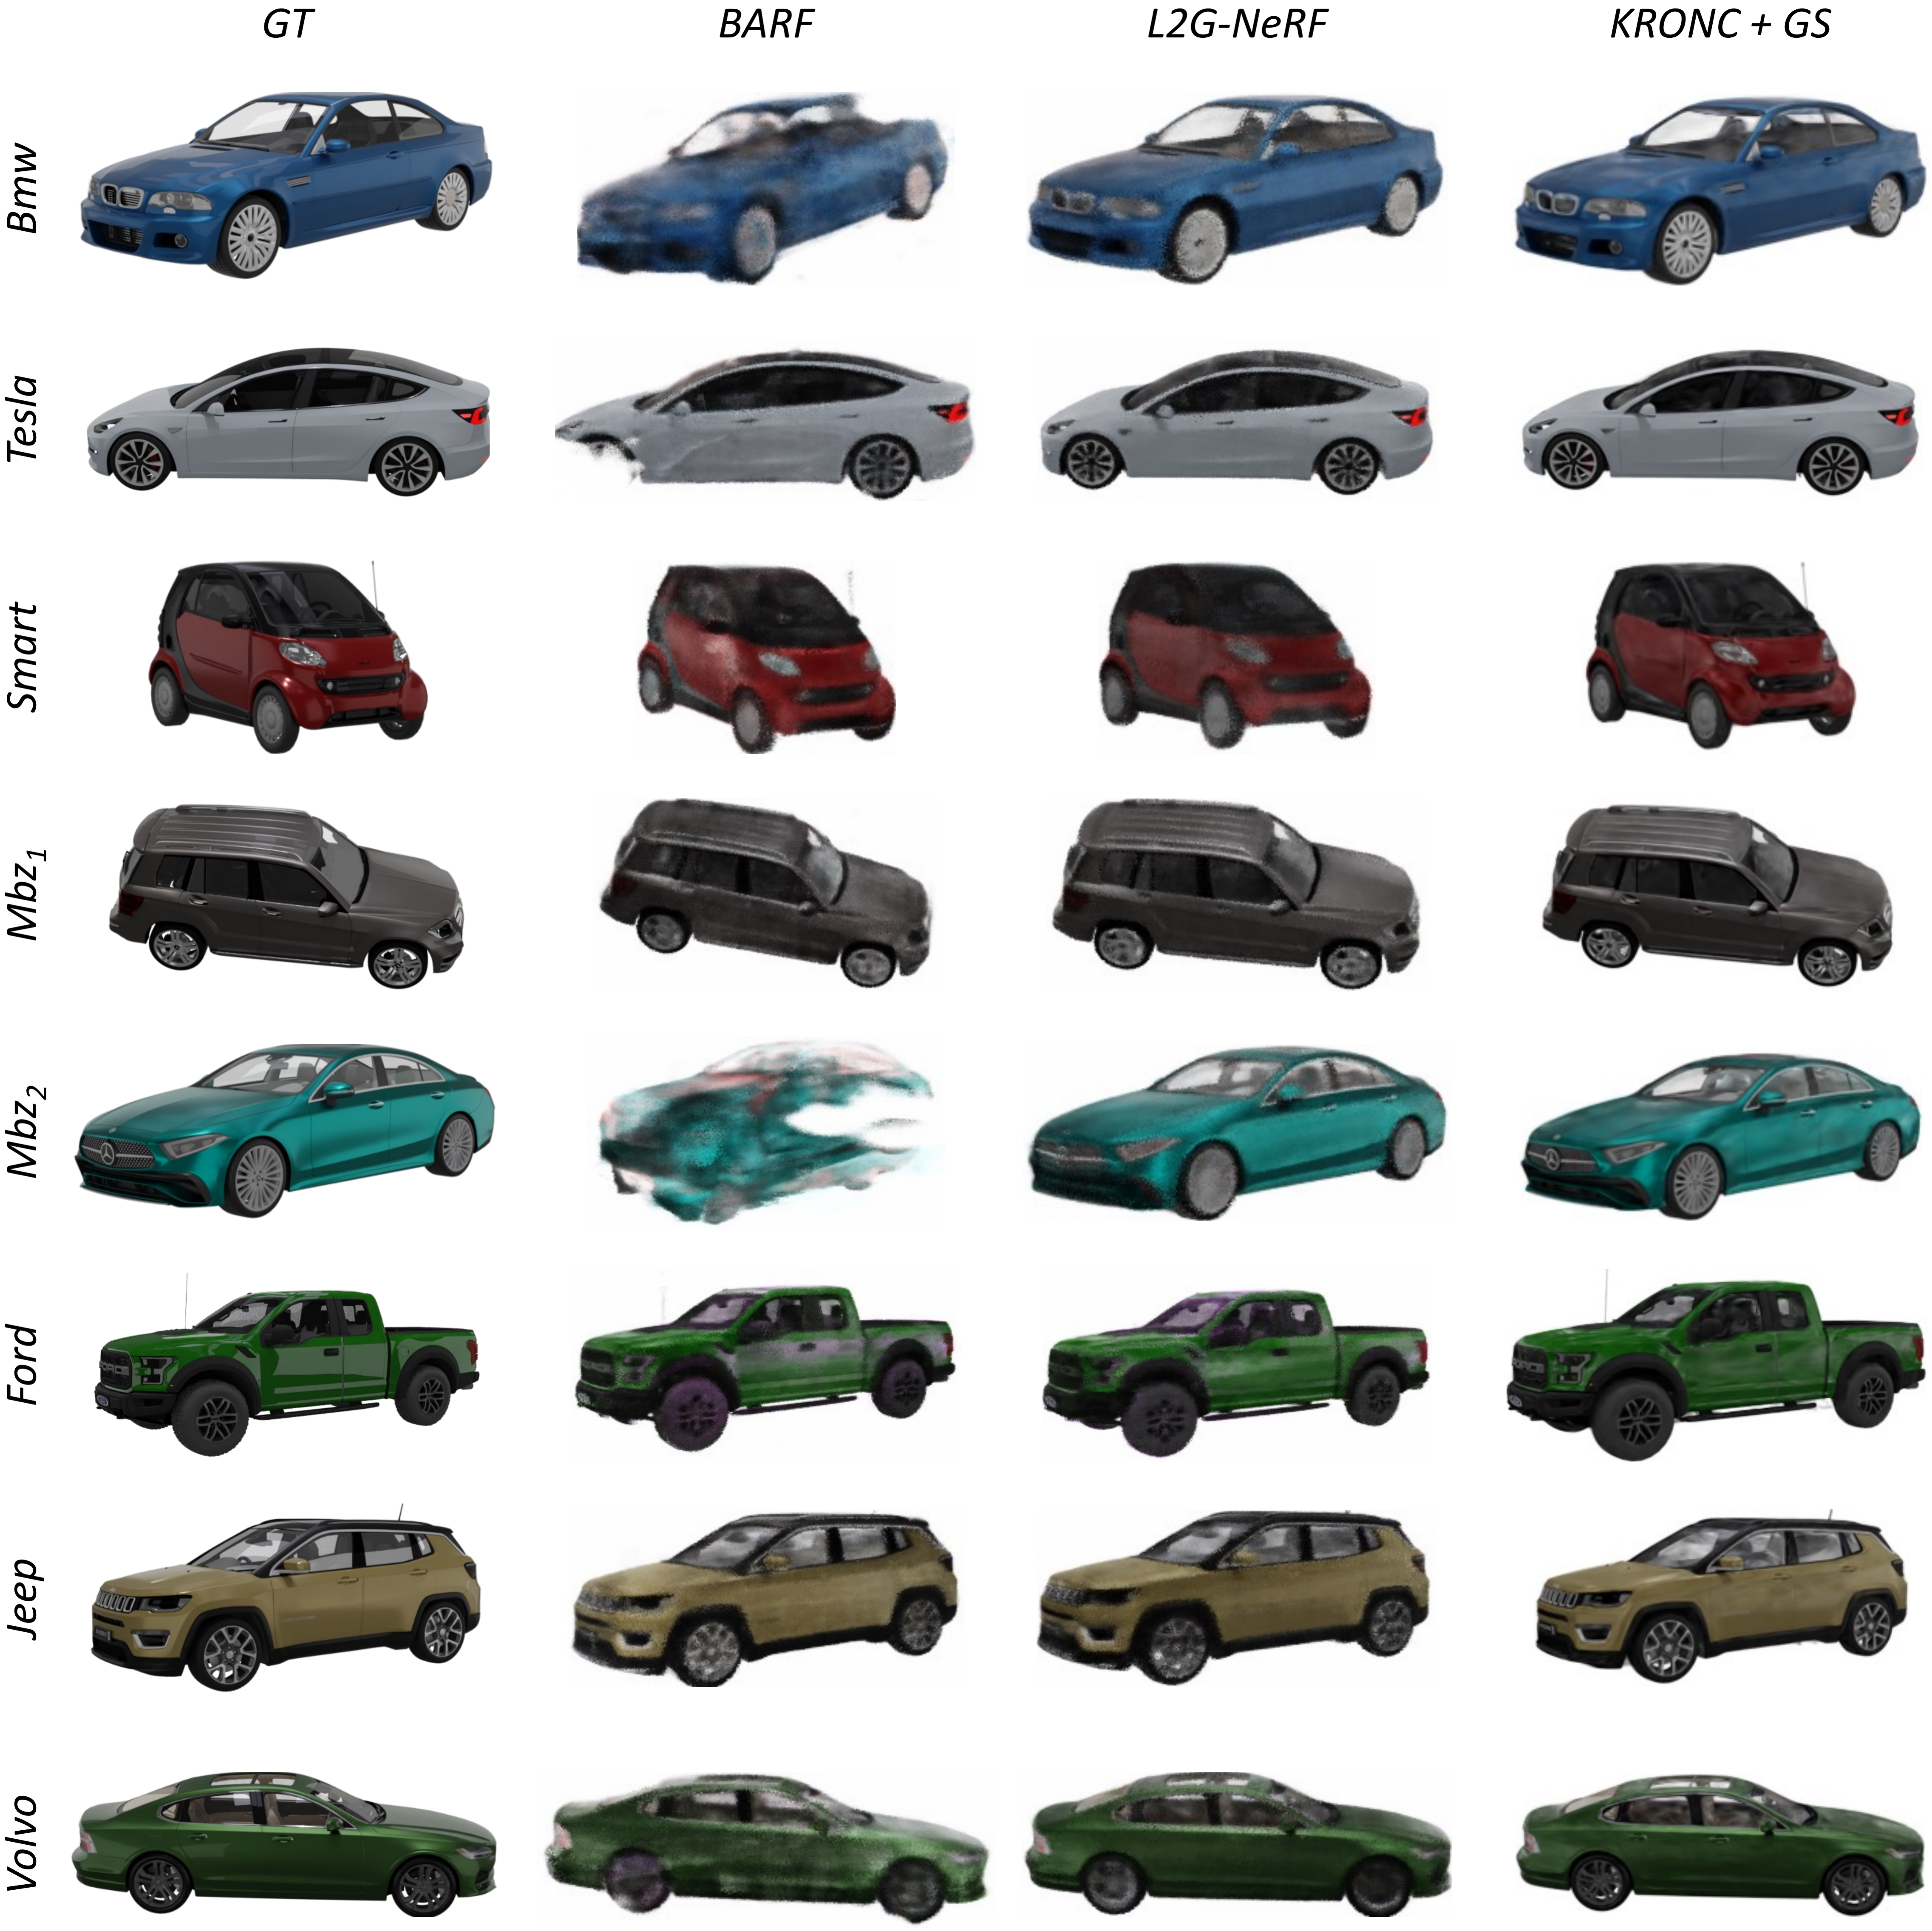

Supplement: Supplementary file 2 [file supp_synt_qualitative.pdf]
